# Supplementary material for: Calibrated Out-of-Distribution Detection with a Generic Representation
Source: arXiv:2303.13148 source file (2023-09-05)
Supplement: Supplementary file 1 [file ood_results_supp.tex]

\begin{table}[ht]\centering\tiny\resizebox{\textwidth}{!}{
\begin{tabular}{lcclllllllll}
\toprule
    {} & {} & {} & \multicolumn{8}{c}{FPR at $95\%$ TPR $\downarrow$ $\biggm/$ AUROC $\uparrow$} & \multirow{2}{*}{{Average}} \\
 
\cmidrule(lr){4-11}

arch & pre-trained & classif &
\multicolumn{1}{c}{SVHN} & 
\multicolumn{1}{c}{MNIST} & 
\multicolumn{1}{c}{Textures} & 
\multicolumn{1}{c}{Places365} & 
\multicolumn{1}{c}{CIFAR-100} & 
\multicolumn{1}{c}{iNaturalist} & 
\multicolumn{1}{c}{TIN} & 
\multicolumn{1}{c}{LSUN} & 
{} \\ 

\midrule

\multirow{4}{*}{Resnet50} & \multirow{2}{*}{ImageNet} & LP & 10.23 / 97.90   & 11.86 / 97.71   & 78.24 / \pz83.32   & 60.51 / \pz86.03   & 59.62 / 87.28 & 97.47 / \pz70.15   & 63.95 / 83.37   & 62.85 / \pz87.05   & 55.59 / 86.60 \\
                          &                           & NM & 97.18 / 63.18   & 69.27 / 92.77   & \pz0.00 / \pz99.96 & \pz0.52 / \pz99.73 & 77.02 / 73.01 & \pz0.01 / \pz99.88 & 47.50 / 90.31   & \pz0.11 / \pz99.82 & 36.45 / 89.83 \\
                          & \multirow{2}{*}{CLIP}     & LP & 10.00 / 98.21   & 13.55 / 97.35   & 75.98 / \pz76.83   & 76.92 / \pz76.24   & 62.70 / 85.53 & 98.80 / \pz56.03   & 72.95 / 78.31   & 64.58 / \pz86.76   & 59.44 / 81.91 \\
                          &                           & NM & 46.26 / 92.75   & \pz4.77 / 97.77 & \pz0.00 / \pz99.95 & \pz0.00 / \pz99.99 & 81.30 / 68.87 & \pz0.01 / \pz99.99 & \pz8.24 / 98.29 & \pz0.00 / 100.00   & 17.57 / 94.70 \\
\cmidrule(lr){4-12}
\multirow{4}{*}{VIT-B/16} & \multirow{2}{*}{ImageNet} & LP & 18.46 / 97.09   & \pz4.42 / 98.57 & 23.94 / \pz96.09   & 17.95 / \pz95.84   & 26.19 / 94.72 & 26.15 / \pz95.57   & 21.94 / 94.39   & \pz8.07 / \pz98.17 & 18.39 / 96.31 \\
                          &                           & NM & 43.93 / 93.51   & \pz1.10 / 99.51 & \pz9.75 / \pz97.87 & \pz9.88 / \pz97.90 & 52.61 / 87.28 & \pz2.91 / \pz99.43 & 40.09 / 89.64   & \pz7.56 / \pz98.82 & 20.98 / 95.50 \\
                          & \multirow{2}{*}{CLIP}     & LP & \pz1.57 / 99.08 & \pz0.02 / 99.85 & 18.55 / \pz96.37   & 57.12 / \pz82.90   & 25.70 / 94.77 & 30.45 / \pz94.97   & 38.19 / 87.69   & 33.09 / \pz93.86   & 25.59 / 93.69 \\
                          &                           & NM & \pz0.07 / 99.74 & \pz3.09 / 97.69 & \pz0.00 / 100.00   & \pz0.00 / 100.00   & 63.59 / 84.56 & \pz0.00 / 100.00   & \pz0.92 / 99.63 & \pz0.00 / 100.00   & \pz8.46  / 97.70 \\
\cmidrule(lr){4-12}
\multirow{2}{*}{VIT-L/16} & \multirow{2}{*}{ImageNet} & LP & 25.79 / 95.79   & 43.38 / 94.44   & \pz9.02 / \pz98.13 & 16.90 / \pz96.04   & 23.01 / 94.85 & 29.61 / \pz94.40   & 17.52 / 95.32   & \pz4.35 / \pz98.85 & 21.20 / 95.98 \\
                          &                           & NM & 96.01 / 77.19   & 84.53 / 85.86   & 52.23 / \pz86.50   & 55.34 / \pz84.52   & 79.62 / 72.80 & 38.19 / \pz92.76   & 77.98 / 71.02   & 70.79 / \pz81.15   & 69.34 / 81.48 \\
\cmidrule(lr){4-12}
\multirow{2}{*}{VIT-L/14} & \multirow{2}{*}{CLIP}     & LP & \pz0.95 / 99.30 & \pz0.25 / 99.68 & \pz4.11 / \pz98.46 & 16.84 / \pz94.08   & 10.89 / 97.50 & \pz8.29 / \pz97.73 & 21.73 / 91.46   & \pz6.78 / \pz97.85 & \pz8.73 / 97.01 \\
                          &                           & NM & \pz0.03 / 99.71 & \pz0.81 / 98.71 & \pz0.00 / 100.00   & \pz0.00 / 100.00   & 65.83 / 86.74 & \pz0.00 / 100.00   & \pz2.27 / 99.35 & \pz0.00 / 100.00   & \pz8.62 / 98.06 \\

\bottomrule
\end{tabular}
}
\caption{Comparison of different architectures and pre-training data --  OOD problems with mixed semantic and domain shifts. The measures are described in the main paper.}
\label{tab:ood_results_supp}
\end{table}
