# Supplementary material for: Calibrated Out-of-Distribution Detection with a Generic Representation
Source: arXiv:2303.13148 source file (2023-09-05)
Supplement: Supplementary file 2 [file osr_results_supp.tex]

\begin{table}[ht]\centering\tiny\resizebox{\textwidth}{!}{
\begin{tabular}{lccccccccc}
\toprule
{} & {} & {} & \multicolumn{6}{c}{AUROC $\uparrow$ $\biggm/$ OSCR $\uparrow$} & \multirow{2}{*}{{Average}} \\

\cmidrule(lr){4-9}

    arch & pre-trained  & classif &
\multicolumn{1}{c}{MNIST} & 
\multicolumn{1}{c}{SVHN} & 
\multicolumn{1}{c}{CIFAR10} & 
\multicolumn{1}{c}{CIFAR+10} & 
\multicolumn{1}{c}{CIFAR+50} & 
\multicolumn{1}{c}{TIN} & 
{} \\ 

\midrule

\multirow{4}{*}{Resnet50}   & \multirow{2}{*}{ImageNet} & LP & 91.82$\pm$1.45 / 90.84$\pm$1.51 & 68.37$\pm$2.24 / 51.22$\pm$2.95 & 89.19$\pm$2.82 / 84.21$\pm$2.24 & 94.30$\pm$2.10 / 90.92$\pm$2.78 & 92.53$\pm$1.13 / 89.19$\pm$1.69 & 88.52$\pm$0.99 / 81.27$\pm$2.57 & 87.46$\pm$1.79 / 81.28$\pm$2.29 \\
                            &                           & NM & 76.84$\pm$2.92 / 62.59$\pm$1.78 & 50.51$\pm$3.02 / 20.93$\pm$2.84 & 81.57$\pm$0.63 / 71.14$\pm$2.01 & 89.57$\pm$0.44 / 82.22$\pm$1.40 & 88.82$\pm$2.17 / 81.50$\pm$0.66 & 80.30$\pm$0.80 / 70.20$\pm$2.84 & 77.94$\pm$1.66 / 64.76$\pm$1.92 \\
                            & \multirow{2}{*}{CLIP}     & LP & 90.57$\pm$1.78 / 88.91$\pm$1.84 & 65.96$\pm$1.76 / 47.37$\pm$1.44 & 87.16$\pm$2.86 / 81.49$\pm$2.17 & 94.74$\pm$3.53 / 91.12$\pm$4.07 & 93.42$\pm$1.36 / 89.86$\pm$1.94 & 82.16$\pm$1.30 / 74.11$\pm$2.71 & 85.67$\pm$2.10 / 78.81$\pm$2.36 \\
                            &                           & NM & 72.29$\pm$4.32 / 59.35$\pm$2.14 & 51.09$\pm$1.24 / 18.71$\pm$1.81 & 73.90$\pm$4.13 / 61.98$\pm$1.96 & 88.82$\pm$1.13 / 80.20$\pm$1.68 & 83.88$\pm$2.99 / 75.72$\pm$2.30 & 69.84$\pm$1.99 / 55.29$\pm$3.44 & 73.30$\pm$2.63 / 58.54$\pm$2.22 \\
\cmidrule(lr){4-10}
 \multirow{4}{*}{VIT-B/16}  & \multirow{2}{*}{ImageNet} & LP & 93.10$\pm$2.06 / 91.82$\pm$2.14 & 65.59$\pm$1.32 / 46.49$\pm$3.12 & 96.07$\pm$0.94 / 93.25$\pm$1.45 & 98.09$\pm$1.95 / 96.27$\pm$2.46 & 97.19$\pm$1.55 / 95.35$\pm$2.03 & 97.07$\pm$0.14 / 93.05$\pm$1.31 & 91.19$\pm$1.33 / 86.04$\pm$2.09 \\
                            &                           & NM & 84.78$\pm$2.01 / 74.61$\pm$0.64 & 50.19$\pm$1.56 / 18.93$\pm$1.09 & 93.66$\pm$0.39 / 88.89$\pm$1.04 & 97.24$\pm$0.90 / 94.32$\pm$1.76 & 97.11$\pm$0.39 / 94.18$\pm$1.10 & 87.69$\pm$1.65 / 82.68$\pm$2.82 & 85.11$\pm$1.15 / 75.60$\pm$1.41 \\
                            & \multirow{2}{*}{CLIP}     & LP & 98.17$\pm$0.30 / 97.40$\pm$0.33 & 71.73$\pm$2.28 / 55.41$\pm$3.56 & 96.82$\pm$0.63 / 94.42$\pm$0.92 & 98.44$\pm$0.86 / 96.85$\pm$1.17 & 97.24$\pm$0.77 / 95.67$\pm$0.44 & 91.40$\pm$0.88 / 86.00$\pm$1.87 & 92.30$\pm$0.95 / 87.63$\pm$1.38 \\
                            &                           & NM & 74.47$\pm$1.50 / 63.90$\pm$2.25 & 53.48$\pm$0.53 / 30.52$\pm$0.60 & 88.80$\pm$2.52 / 84.46$\pm$1.68 & 94.14$\pm$1.20 / 91.22$\pm$1.55 & 91.87$\pm$1.85 / 89.01$\pm$1.56 & 84.75$\pm$1.33 / 74.92$\pm$2.73 & 81.25$\pm$1.49 / 72.34$\pm$1.73 \\
\cmidrule(lr){4-10}
\multirow{2}{*}{VIT-L/16}   & \multirow{2}{*}{ImageNet} & LP & 92.48$\pm$2.07 / 91.16$\pm$2.30 & 69.20$\pm$3.08 / 50.64$\pm$5.40 & 95.97$\pm$1.07 / 93.17$\pm$1.32 & 98.45$\pm$1.15 / 96.60$\pm$1.64 & 96.97$\pm$0.87 / 95.01$\pm$1.41 & 97.87$\pm$0.14 / 94.93$\pm$1.18 & 91.82$\pm$1.40 / 86.92$\pm$2.21 \\
                            &                           & NM & 82.82$\pm$2.25 / 72.94$\pm$0.62 & 50.62$\pm$1.43 / 22.02$\pm$2.44 & 81.15$\pm$1.24 / 76.73$\pm$2.32 & 85.88$\pm$1.38 / 83.09$\pm$1.94 & 86.99$\pm$0.72 / 84.16$\pm$1.16 & 78.54$\pm$2.92 / 75.35$\pm$3.77 & 77.67$\pm$1.66 / 69.05$\pm$2.04 \\
\cmidrule(lr){4-10}
\multirow{2}{*}{VIT-L/14}   & \multirow{2}{*}{CLIP}     & LP & 97.40$\pm$0.57 / 96.76$\pm$0.61 & 78.32$\pm$0.65 / 65.61$\pm$1.10 & 98.28$\pm$0.60 / 97.08$\pm$1.00 & 99.32$\pm$0.38 / 98.50$\pm$0.50 & 98.15$\pm$0.15 / 97.36$\pm$0.22 & 94.64$\pm$0.62 / 91.27$\pm$1.66 & 94.35$\pm$0.50 / 91.10$\pm$0.85 \\
                            &                           & NM & 84.44$\pm$1.28 / 76.86$\pm$1.36 & 57.73$\pm$1.69 / 41.94$\pm$2.03 & 90.93$\pm$1.31 / 88.61$\pm$1.05 & 93.79$\pm$1.40 / 92.12$\pm$1.90 & 93.46$\pm$0.55 / 91.78$\pm$0.62 & 89.92$\pm$1.53 / 84.23$\pm$2.15 & 85.05$\pm$1.29 / 79.26$\pm$1.52 \\

\bottomrule
\end{tabular}
}
\caption{Comparison of different architectures and pre-training data -- OOD problems with semantic shift only. The measures are described in the main paper.}
\label{tab:osr_results_supp}
\end{table}
